# Supplementary material for: Independently Tunable Flat Bands and Correlations in a Graphene Double Moir\'e System
Source: arXiv:2411.18785 source file (2024-11-27)
Supplement: Supplementary file 1 [file SM.pdf]

# Supplemental Material: Independently Tunable Flat Bands and Correlations in a Graphene Double Moiré System

Yimeng Wang, Jihang Zhu, G. William Burg, Anand Swain, Kenji Watanabe,
Takashi Taniguchi, Yuebing Zheng, Allan H. MacDonald, Emanuel Tutuc

## Sample Fabrication

The double moiré samples are fabricated with the ‘cut-and-stack’ method. The hexagonal boron nitride (hBN) and graphene flakes are mechanically exfoliated onto Si/$SiO_2$ ($285\,\mathrm{nm}$) substrate and inspected by optical microscopy. Two graphene flakes are cut into two sections with supercontinuum laser (SuperK FIANIUM FIU-15, 40-50% power). The topmost hBN flake is picked up by polypropylene carbonate spin-coated on a hemispherical polydimethylsiloxane handle. One section of the first graphene flake is then picked up by the hBN and the remaining section is rotated with a small angle and sequentially picked up. The same process is repeated for the second graphene flake. The straight edges of the two graphene flakes are identified and intentionally misaligned to form a $> 5^\circ$ angle. The stack is then released onto the bottom-gate structure composed of a hBN/graphite stack on Si/$SiO_2$ substrate prepared in advance. The resulting stack is then etched with $CHF_3$ and $O_2$ plasma to define the Hall-bar shape, followed by metal deposition (Cr/Pd/Au) to define the top gate and form edge contacts.

## Measurement Setup

The measurements are performed in a dilution refrigerator with a base temperature of $95\,\mathrm{mK}$. Standard low-frequency lock-in techniques are used with an excitation current of 0.5-$1\,\mathrm{nA}$ and an excitation frequency of $7.31\,\mathrm{Hz}$. Four-point measurement configurations are adopted for all the resistance measurements.

## I. Electrostatic Analysis

This section provides information on the electrostatic analysis which leads to Eq. 1 in the main text. Figure S1 shows the schematic of the band alignment in the double moiré system. As discussed in the main text, the two constituent TBGs in a double moiré sample have independent moiré bands that are only capacitively coupled. The applied top and bottom gate biases

are $V_{\mathrm{TG}}$ and $V_{\mathrm{BG}}$, respectively, and the channel is shorted to ground. $V_{\epsilon,\mathrm{T}}$, $V_{\epsilon,\mathrm{IL}}$, and $V_{\epsilon,\mathrm{B}}$ denote the changes in electrostatic potential across the top gate dielectric, between the two constituent TBGs, and across the bottom gate dielectric, respectively. An applied $V_{\mathrm{BG}}$ changes the electrostatic potential drop across the bottom gate dielectric as well as the chemical potential of the bottom TBG,

$$eV_{\mathrm{BG}} = eV_{\epsilon,\mathrm{B}} + \mu_{\mathrm{B}}, \tag{S1}$$

Similarly,

$$\begin{aligned} 0 &= -eV_{\epsilon,\mathrm{IL}} + \mu_{\mathrm{B}} - \mu_{\mathrm{T}}, \\ eV_{\mathrm{TG}} &= eV_{\epsilon,\mathrm{T}} + \mu_{\mathrm{T}}, \end{aligned} \tag{S2}$$

The electrostatic potential drives the charge transfers,

$$\begin{aligned} C_{\mathrm{BG}}V_{\epsilon,\mathrm{B}} &= -en_{\mathrm{BG}}, \\ C_{\mathrm{IL}}V_{\epsilon,\mathrm{IL}} &= -e(n_{\mathrm{B}} + n_{\mathrm{BG}}), \\ C_{\mathrm{TG}}V_{\epsilon,\mathrm{T}} &= e(n_{\mathrm{T}} + n_{\mathrm{B}} + n_{\mathrm{BG}}), \end{aligned} \tag{S3}$$

$n_{\mathrm{T}}$, $n_{\mathrm{B}}$ and $n_{\mathrm{BG}}$ are the carrier density in the top TBG, bottom TBG, and bottom gate, respectively. Combining Eq. S1-S3, Eq. 1 in the main text can be obtained,

$$\begin{aligned} V_{\mathrm{BG}}C_{\mathrm{BG}} &= en_{\mathrm{B}} + \frac{\mu_{\mathrm{B}}}{e}(C_{\mathrm{BG}} + C_{\mathrm{IL}}) - \frac{\mu_{\mathrm{T}}}{e}C_{\mathrm{IL}}\ , \\ V_{\mathrm{TG}}C_{\mathrm{TG}} &= en_{\mathrm{T}} + \frac{\mu_{\mathrm{T}}}{e}(C_{\mathrm{TG}} + C_{\mathrm{IL}}) - \frac{\mu_{\mathrm{B}}}{e}C_{\mathrm{IL}}\ . \end{aligned} \tag{S4}$$

## II. Capacitance Extraction

It is important to determine the capacitance of the top and bottom gate dielectric carefully since the capacitance values are crucial part in the thermodynamic equations. To that end, we utilize the magneto-transport data to accurately determine the carrier density associated with Landau level fillings in each constituent TBGs in the double moiré.

Figure S2 shows the longitudinal resistance plotted as a function of top and bottom gate biases measured in a perpendicular magnetic field $B = 3\,\mathrm{T}$. The resistance minima along the

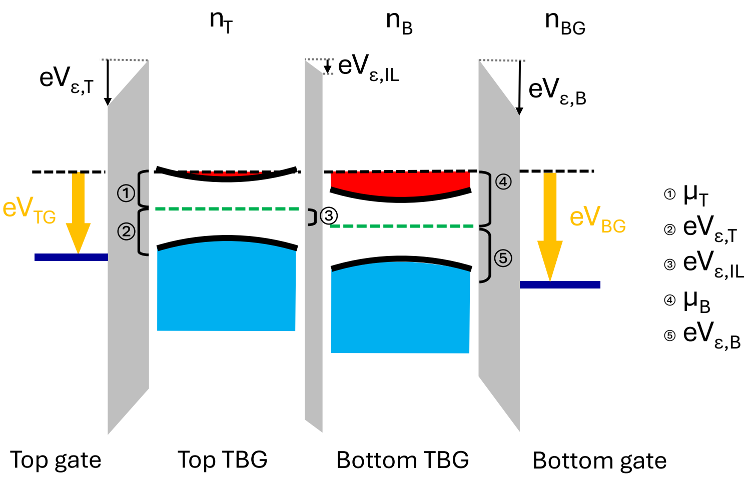


Figure S1: Band diagram of the double moiré system. The black dashed line marks the ground potential. Green dashed lines mark the zero chemical potential of the constituent TBGs in the double moiré.

$V_{\mathrm{BG}}$ and $V_{\mathrm{TG}}$ axes are associated with Landau level fillings (with integer Landau level index $N$) of the top and bottom TBGs, respectively. In Fig. S2(b), the Landau levels are marked with green dashed lines, and adjacent Landau levels have a filling factor difference $\Delta N = 4$ for each constituent TBGs. From the quantum Hall state marked by the upper left orange dot to the lower right, the change of the Landau level filling factor indices are +16 and -16 for the top and bottom TBG, respectively. Applying Eq. 1 in the main text, because $\Delta n_{\mathrm{T}} = -\Delta n_{\mathrm{B}}$,

$$\Delta V_{\mathrm{TG}} C_{\mathrm{TG}} + \Delta V_{\mathrm{BG}} C_{\mathrm{BG}} = \frac{\Delta \mu_{\mathrm{T}}}{e} C_{\mathrm{TG}} + \frac{\Delta \mu_{\mathrm{B}}}{e} C_{\mathrm{BG}}. \tag{S5}$$

Because $\frac{\Delta \mu_{\mathrm{T}}}{e} << \Delta V_{\mathrm{TG}}$ and $\frac{\Delta \mu_{\mathrm{B}}}{e} << \Delta V_{\mathrm{BG}}$, the ratio of the top and bottom gate capacitance $C_{\mathrm{TG}}/C_{\mathrm{BG}} = -\Delta V_{\mathrm{BG}}/\Delta V_{\mathrm{TG}}$. Here we made the assumption that the capacitance values do not change with $B$-field, which can be substantiated with our observation that the slopes of the resistance peaks are constant when $B$-field is varied (Eq. 2 in the main text).

We then determine the values of the capacitance with the data in Fig. S3(a), which shows the longitudinal resistance as a function of the carrier density and the perpendicular magnetic field.

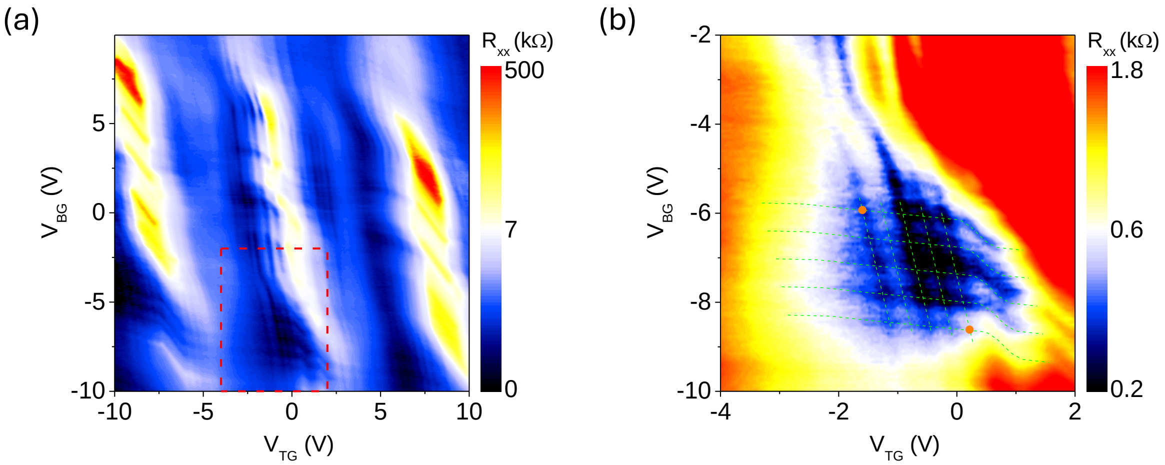


Figure S2: (a) $R_{\mathrm{xx}}$ vs. $V_{\mathrm{TG}}$ and $V_{\mathrm{BG}}$ measured in perpendicular magnetic field $3\,\mathrm{T}$. (b) An expansion of data in the dashed rectangle in (a). Longitudinal (latitudinal) green dashed lines mark the quantum Hall states of the top (bottom) TBGs with $\Delta N = 4$ interval. Data is taken at $T = 95\,\mathrm{mK}$.

The data is taken along the red line in Fig. S3(b) to match the zero density loci for the bottom TBG. Therefore total carrier density plotted as the x-axis in Fig. S3(a) equals to the carrier density in the top TBG. We observe Landau fans similar to what is usually observed in single moiré systems which can be fitted with the equation $n/n_{\mathrm{s}} = (N/4)(\phi/\phi_0) + s$ to determine the carrier density and hence the top and bottom gate capacitances. Here, $n_{\mathrm{s}}$ is the full filling carrier density for the top TBG at $\nu_{\mathrm{T}} = 1$, $\phi = BA$ is the magnetic flux per moiré unit cell, $\phi_0$ is the magnetic flux quanta $h/e$ with $h$ the Planck constant, and $s$ is the integer index for the moiré subband filling in the top TBG. In sample S4, the capacitance is determined to be $C_{\mathrm{TG}} = 143\,\mathrm{nF/cm^2}$ and $C_{\mathrm{BG}} = 97\,\mathrm{nF/cm^2}$. With the top and bottom gate capacitance values known, the interlayer capacitance and the gap sizes can then be determined following Eq. 2 in the main text.

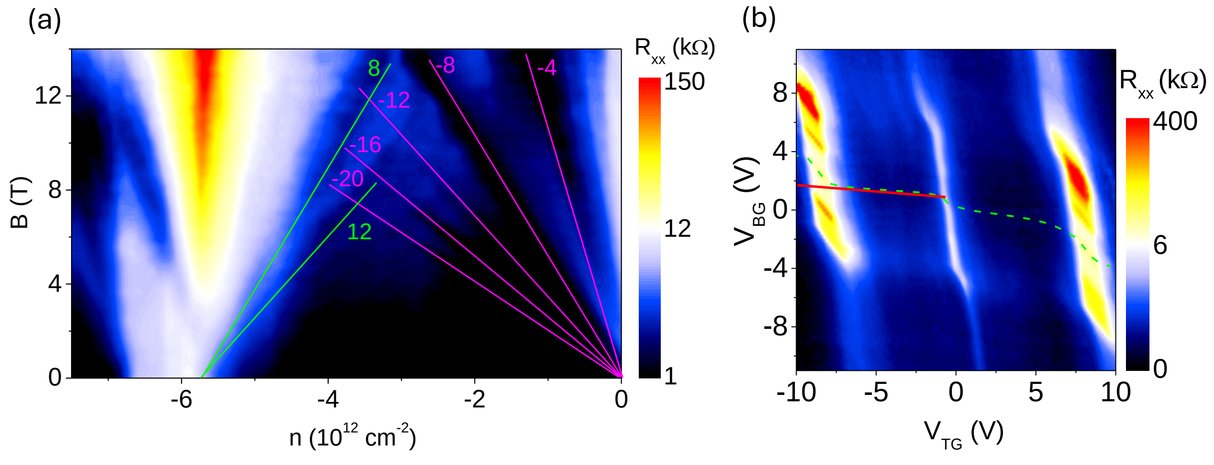


Figure S3: **a** $R_{\rm xx}$ vs. $n$ and $B$ with Landau fans taken in sample S4. Numbers label the Landau level indices. The data is taken along the red solid line in **b**. **b** $R_{\rm xx}$ vs. $V_{\rm TG}$ and $V_{\rm BG}$ at $0\,{\rm T}$, green dashed line marks the zero carrier density loci for the bottom TBG.

## III. Extraction of Constant Chemical Potential

This section focuses on the extraction of constant chemical potential loci with $R_{\rm xx}$ vs. $V_{\rm TG}$ and $V_{\rm BG}$ data measured in double moiré samples. As explained in the main text, in ($V_{\rm TG}$, $V_{\rm BG}$) plane, the incompressible states of the two constituent TBGs form a pattern depicted by Fig. 2(b). By tracing the boundary between the compressible and incompressible states, the constant chemical loci can be obtained at the filling factors where the constituent TBG is incompressible. Here we take the sample S2 as an example, and explain the procedure in detail. Figure S4 show the $R_{\rm xx}$ plotted in the ($V_{\rm TG}$, $V_{\rm BG}$) plane. As shown in Fig. S4(a) and (e), the incompressible states of the top TBG can be traced by the sharp peaks along the y-axis [green lines in Fig. S4(e)]. For all the filling factors where the top TBG is incompressible (shown in Fig. S4(e) with $\nu_{\rm T} = 0$ and $1/2$ as examples), the peaks follow the same shape. Thus the constant chemical potential loci can be traced at any incompressible filling factor. Similarly, the constant chemical potential loci of the bottom TBG can be obtained by tracing the resistance peak at bottom TBG incompressible states. However, the resistance peaks only appear at $\nu_{\rm B} = 0, \pm 1$ due to the

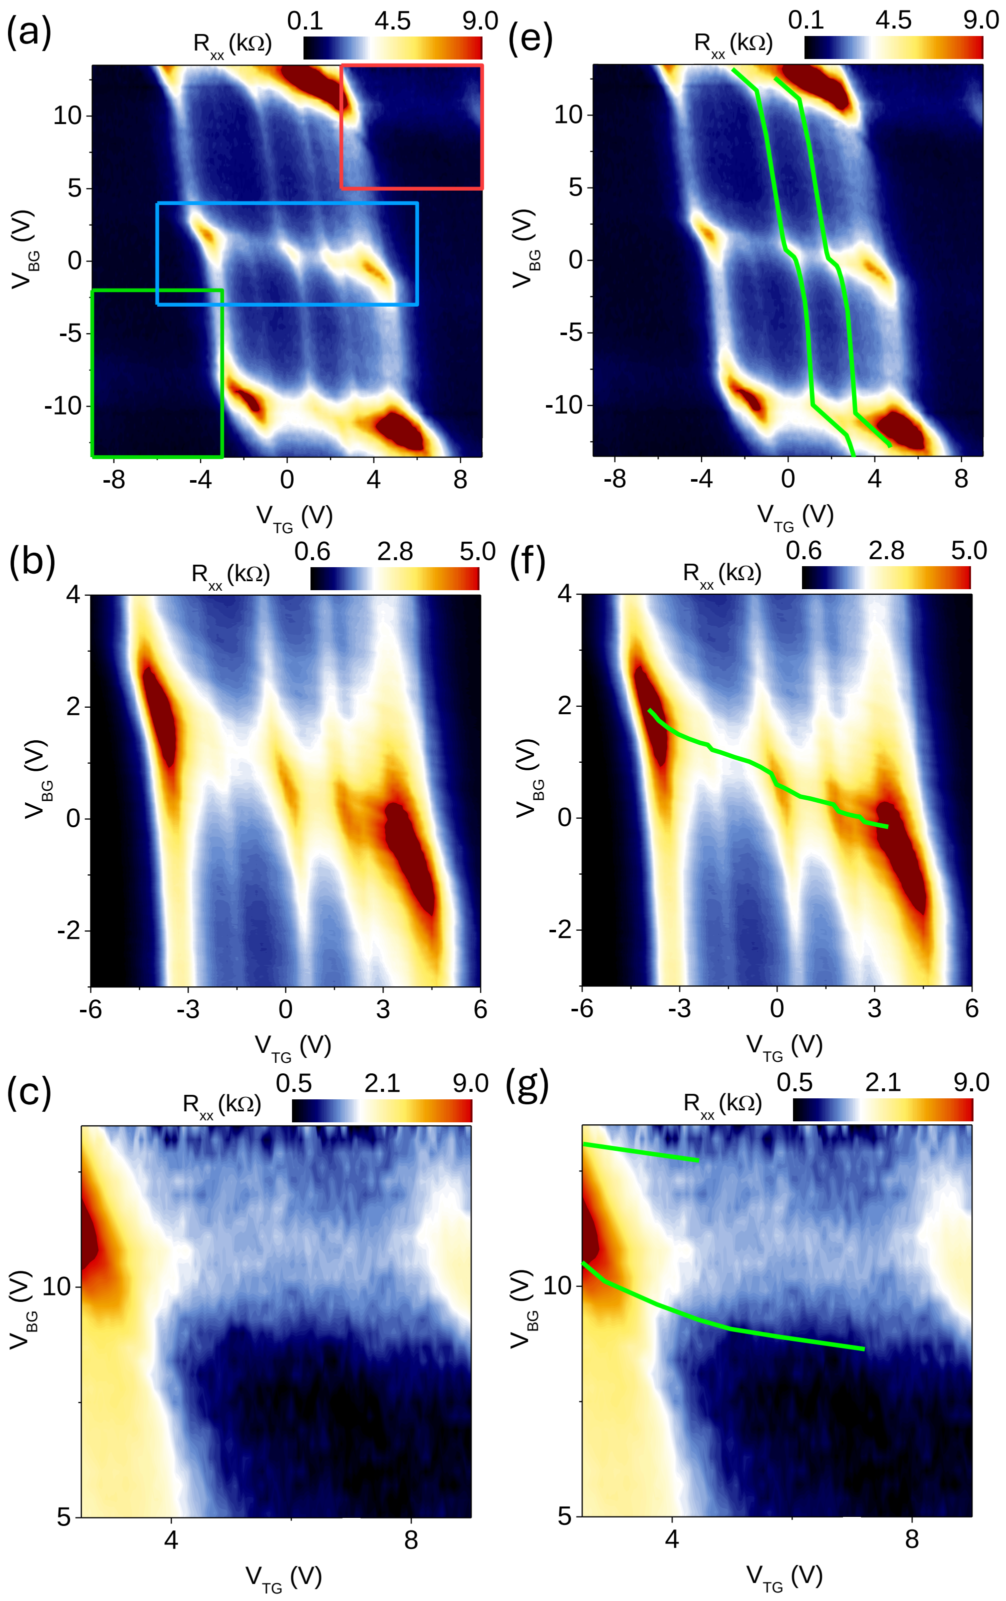
(a)
(b)
(c)
(e)
(f)
(g)
$R_{xx}$ (kΩ)
0.1 4.5 9.0
0.6 2.8 5.0
0.5 2.1 9.0
$V_{BG}$ (V)
$V_{TG}$ (V)

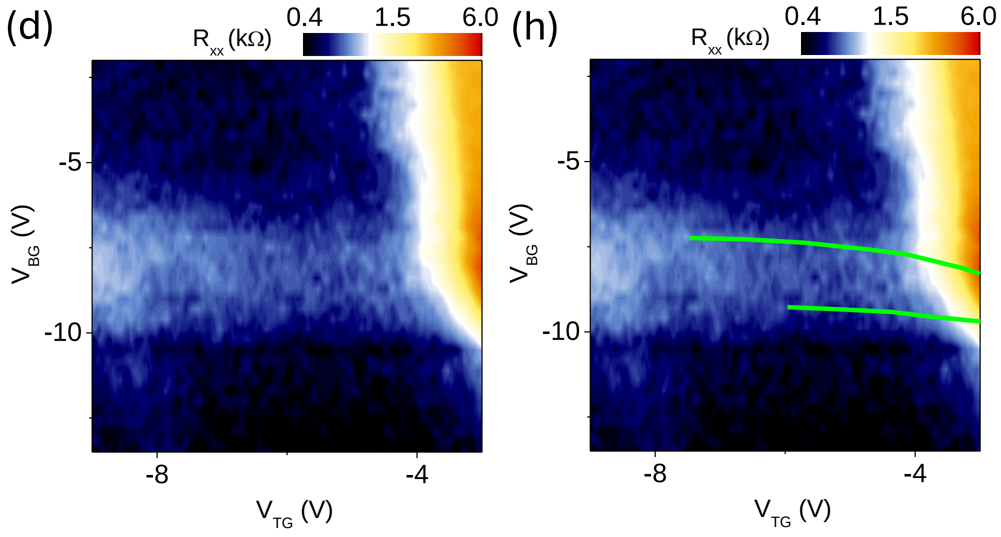


Figure S4: (a) $R_{\rm xx}$ vs. $V_{\rm TG}$ and $V_{\rm BG}$ measured in sample S2 with $\theta_{\rm T} = 0.95°$ and $\theta_{\rm B} = 1.54°$. (b)-(d) Expanded view of data in (a) marked by the (b) blue, (c) red and (d) green rectangles. (e)-(h) Data in (a)-(d) with constant chemical potential loci for the (e) top and (f-h) bottom TBG marked by green curves.

lack of correlated insulators at larger TBG angle, and they are interrupted by multiple peaks from incompressible states of the top TBG. In Fig. S4(b) we show the expanded view of $R_{\rm xx}$ vs. $V_{\rm TG}$ and $V_{\rm BG}$ around the $\nu_{\rm B} = 0$ resistance peak, and the trace of the peak [green trace in Fig. S4(f)] are determined visually by marking the center of the peak for each $V_{\rm TG}$. We note that the incompressible states at $\nu_{\rm T} = 0, \pm 1$ as well as the correlated insulators at $\nu_{\rm T} = \pm 1/2$ enhance the $\nu_{\rm B} = 0$ peak by adding local maxima along y-axis, and when determining the constant chemical potential loci we try to exclude this effect. It can also be seen from Fig. S4(f) that traces of resistance oscillations parallel to the green trace are present above and below the $\nu_{\rm B} = 0$ peak, corroborating the accuracy of the chemical potential loci extracted. In Fig. S4(c)-(d) and (g)-(h) we plot data in Fig. S4(a) with different color scales to show how the constant chemical potential loci at the upper and lower boundary of $\nu_{\rm B} = 1$ with $\nu_{\rm T} > 1$ [Fig. S4(c) and (g)] and $\nu_{\rm B} = -1$ with $\nu_{\rm T} < -1$ [Fig. S4(d) and (h)] are determined.

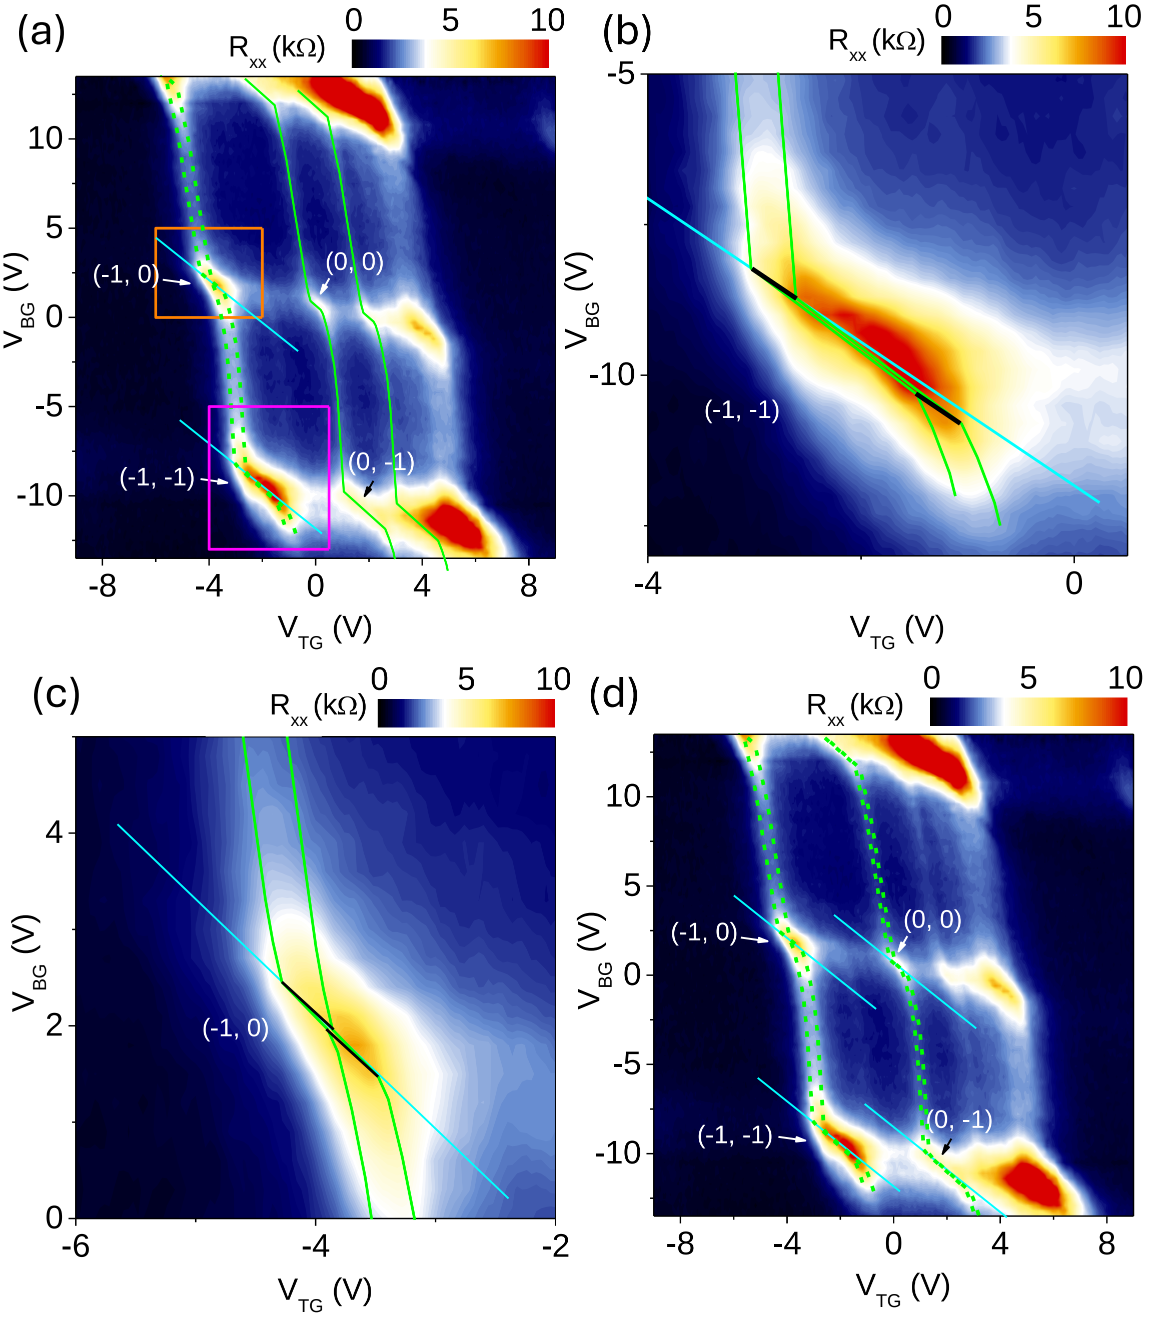


Figure S5: $R_{\rm xx}$ vs. $V_{\rm TG}$ and $V_{\rm BG}$ measured in sample S2. (a), (d) Solid green lines are constant chemical potential loci for the top TBG, same as in Fig. S4. The dashed lines mark the boundary of the (a) $\nu_{\rm T} = -1$ and (d) $\nu_{\rm T} = 0$ state. Cyan lines mark the slope for the diamond edges associated with the top TBG gap. White numbers labels the $(\nu_{\rm T}, \nu_{\rm B})$ indices for the gapped states. (b)-(c) Expanded view for data in the (b) magenta and (c) orange boxes. Black lines mark the diamond edges that are associated with the top TBG gap at $\nu_{\rm T} = -1$.

We now explain how we match the diamond shape (Fig. 2c) to the $R_{\mathrm{xx}}$ vs. $V_{\mathrm{TG}}$ and $V_{\mathrm{BG}}$ data at the states when both of the TBG subsystems are in gapped states. Starting with the constant $\mu_{\mathrm{T}}$ traces determined in Fig. S4, based on our finding that the two TBG are only weakly coupled, the constant chemical potential loci at the boundary of the gapped $\nu_{\mathrm{T}} = -1$ state can be determined with the following steps: (1) take a copy of the constant $\mu_{\mathrm{T}}$ loci [green solid line in Fig. S5(a)] and place it on one edge of the $\nu_{\mathrm{T}} = -1$ resistance peak [right green dashed line in Fig. S5(a)] ; (2) draw a line with a slope $-\frac{C_{\mathrm{TG}}}{C_{\mathrm{BG}}}(\frac{C_{\mathrm{IL}}}{C_{\mathrm{IL}}+C_{\mathrm{TG}}})$ [cyan solid line in Fig. S5(a)]; (3) make another copy of the constant $\mu_{\mathrm{T}}$ loci, offset it from the first copy along the slope of the cyan line to match the resistance peak at $\nu_{\mathrm{T}} = -1$ [left green dashed line in Fig. S5(a)]. The fixed slope is based on the analysis of Eq. 2 and Fig. 2c. We note that for the state at $\nu_{\mathrm{T}} = 0$, the boundary of the incompressible state should be determined with two constant $\mu_{\mathrm{T}}$ loci offset with a slope $-\frac{C_{\mathrm{TG}}}{C_{\mathrm{BG}}}(\frac{C_{\mathrm{IL}}}{C_{\mathrm{IL}}+C_{\mathrm{TG}}})$ as well. Because the top TBG gaps in these states are small, we utilized the narrow peak to extract the constant $\mu_{\mathrm{T}}$ loci by neglecting the finite peak width, but the width of the peak which corresponds to the charge neutrality gap in the top TBG can be extracted from the constant $\mu_{\mathrm{B}}$ loci shown in Fig. S4(f). Figure S7(d) shows the boundary of the gapped state at $\nu_{\mathrm{T}} = 0$.

Figure S5(b) shows an expanded view of Fig. S5(a) data marked in the magenta box. The segment of the cyan line that forms one edge of the diamond is marked in black, as well as the opposite edge of the diamond. The length of these black edges corresponds to the top TBG gap at $\nu_{\mathrm{T}} = -1$. This gap size can also be found at the $(\nu_{\mathrm{T}}, \nu_{\mathrm{B}}) = (-1, 0)$ state, as shown in Fig. S5(c). We note that the diamond shape in these states can be quite slender, due to similar slope values between the adjacent diamond edges.

Figure S6 shows the $R_{\mathrm{xx}}$ vs. $V_{\mathrm{TG}}$ and $V_{\mathrm{BG}}$ in four double moiré samples. The green solid lines are the constant chemical potential loci at the incompressible states for each constituent TBGs. The signatures of correlated insulating states can be observed in the constituent TBGs

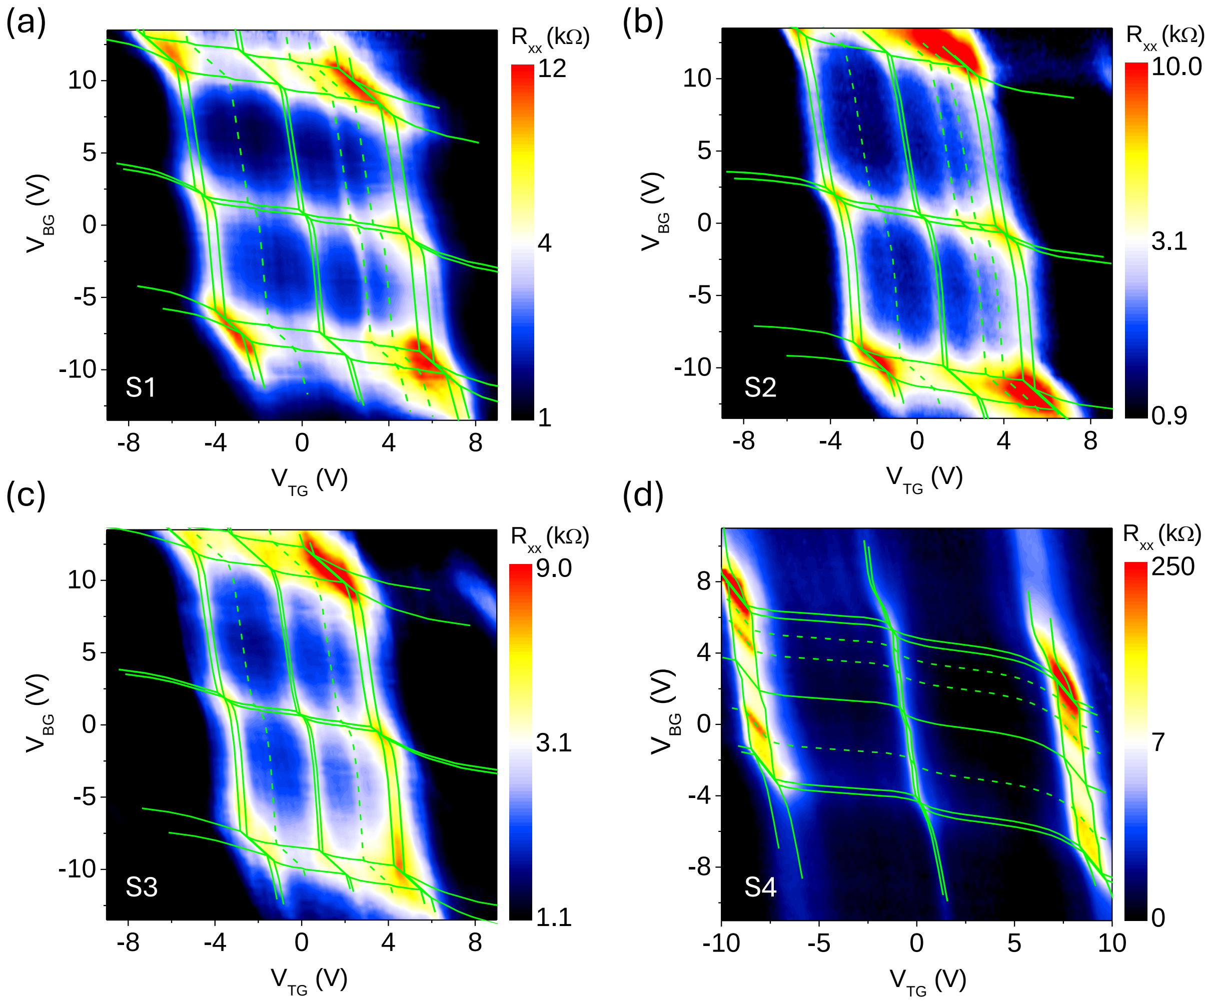


Figure S6: $R_{\mathrm{xx}}$ vs. $V_{\mathrm{TG}}$ and $V_{\mathrm{BG}}$ in four double moiré samples. Solid lines are constant chemical potential loci for the constituent TBGs. Dashed lines mark the constant potential loci where the correlated insulators are observed in the constituent TBGs with twist angles close to the magic angle. Data are taken at $T = 95\,\mathrm{mK}$.

close to the magic angle (0.91°-1.07°) marked by the green dashed lines. The correlated insulators are most prominent when the opposite TBG in the double moiré is in the incompressible states. We note that samples S1-3 are adjacent sections in the same device. We observe a spatial twist angle variation of $0.03° - 0.1°/\mu\mathrm{m}$.

## IV. Discussion on the Charge Neutrality Gap

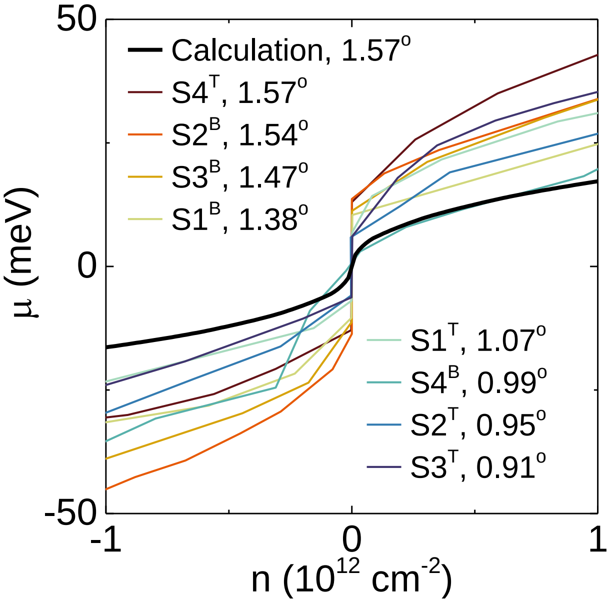


Figure S7: $\mu$ vs. $n$ measured for each TBG in four double moiré samples in comparison with a $\mu \propto \sqrt{n}$ dependence calculated with single-particle model for $\theta = 1.57°$ TBG. The superscripts in the legend label the constituent top (T) and bottom (B) TBGs.

In this section we examine more closely the behavior of the chemical potential around charge neutrality measured in the TBGs in our double moiré samples. Figure S7 shows $\mu$ vs. $n$ data in the vicinity of the charge neutrality, with the black solid line showing the $\mu \propto \sqrt{n}$ dependence in a single-particle calculation for a TBG with $\theta = 1.57°$. The $\mu \propto \sqrt{n}$ can lead to a sharp increase of chemical potential around $n = 0$, with a steeper slope when the Fermi velocity is higher. Compared with the calculation, our experimental data show a more pronounced

change in chemical potential. This suggests that our experimental data reveal either a bona fide gap at charge neutrality or a diverging Fermi velocity near charge neutrality that deviates from the single-particle prediction. We note that it is challenging for any chemical potential or compressibility measurements to distinguish between these two cases.

## V. Bistritzer-MacDonald model parameters

The specific model parameters $\alpha = 0.3$ for $\theta = 0.91°$, $\alpha = 0.6$ for $\theta = 0.99°$ to $1.57°$ and $\alpha = 1.0$ for $\theta = 1.7°$ are chosen to qualitatively match experimental insulating gaps $E_{g,\pm1}$. We have calculated the gaps $E_{g,\pm1}$ and chemical potential changes $\Delta\mu_n$, $\Delta\mu_p$ using various theoretical model parameters commonly used in the literature, as shown in Fig. S8. The legends Fig. S8 represent:

"BM parameter 1": $v_F = 0.86398 \times 10^6$ m/s, $w = 110$ meV, $\alpha = 0.6$, $w_{NL} = -20$ meV.

"parameter 1 large T ratio": $v_F = 0.86398 \times 10^6$ m/s, $w = 110$ meV, $\alpha = 0.8$, $w_{NL} = -20$ meV.

"parameter 1 small T ratio": $v_F = 0.86398 \times 10^6$ m/s, $w = 110$ meV, $\alpha = 0.4$, $w_{NL} = -20$ meV.

"parameter 1 large w$_{NL}$": $v_F = 0.86398 \times 10^6$ m/s, $w = 110$ meV, $\alpha = 0.6$, $w_{NL} = -40$ meV.

"BM parameter 2": $v_F = 0.8 \times 10^6$ m/s, $w = 97.5$ meV, $\alpha = 0.82$, $w_{NL} = -20$ meV [2].

"Fully relaxed model SK": Slater-Koster tight-binding parameters for $\theta = 1.05°$ [1,3].

"Fully relaxed model Wannier": Wannier tight-binding parameters for $\theta = 1.05°$ [1,3].

Our results show that the gaps $E_{g,\pm1}$ are sensitive to $\alpha$, while they exhibit minimal dependence on $w_{NL}$, the Fermi velocity $v_F$ or the magnitude of interlayer tunneling $w$. We hypothesize that the evolution of the gaps with twist angle comes from the twist-angle-dependent corrugation and lattice relaxation effects. However, the exact dependencies of these model pa-

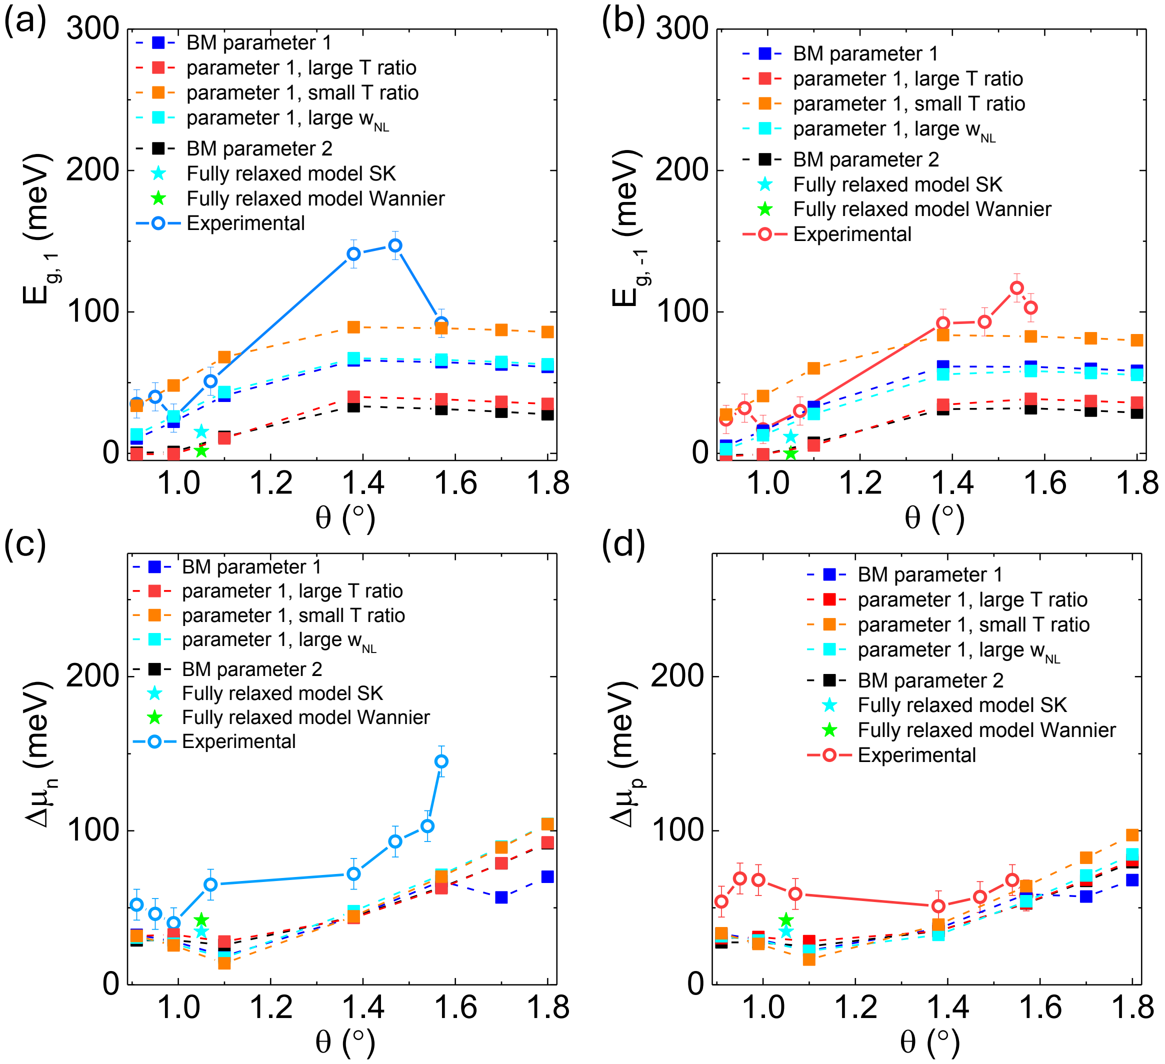


Figure S8: Comparison of (a) $E_{g,1}$, (b) $E_{g,-1}$, (c) $\Delta\mu_n$, and (d) $\Delta\mu_p$ vs. $\theta$ calculated by self-consistent Hartree approximation based on the BM model using different model parameters (dashed lines), and the experimental data (solid lines).

rameters on the twist angle remain unclear. Additionally, interactions with a second adjacent TBG sample could introduce further relaxation effects. For this reason, in the main text, we have chosen a small $\alpha$ for small angles and a large $\alpha$ for large angles to qualitatively match experimental data. While this choice provides reasonable agreement, it is not a rigorous determination.

# References


[1] Jian Kang and Oskar Vafek. Pseudomagnetic fields, particle-hole asymmetry, and microscopic effective continuum hamiltonians of twisted bilayer graphene. Phys. Rev. B, 107:075408, Feb 2023.

[2] Mikito Koshino, Noah F. Q. Yuan, Takashi Koretsune, Masayuki Ochi, Kazuhiko Kuroki, and Liang Fu. Maximally localized wannier orbitals and the extended hubbard model for twisted bilayer graphene. Phys. Rev. X, 8:031087, Sep 2018.

[3] Oskar Vafek and Jian Kang. Continuum effective hamiltonian for graphene bilayers for an arbitrary smooth lattice deformation from microscopic theories. Phys. Rev. B, 107:075123, Feb 2023.
